# Supplementary material for: Non-monotonic motion of sliding droplets on strained soft solids
Source: arXiv:2411.03915 ancillary file (2025-04-12)
Supplement: Supplementary file 1 [file Supplemental.pdf]

# Non-monotonic motion of sliding droplets on strained soft solids

Youchuang Chao,[1,*] Hansol Jeon,[1] and Stefan Karpitschka[1,2,†]

[1] *Max Planck Institute for Dynamics and Self-Organization, Göttingen 37077, Germany*

[2] *Department of Physics, University of Konstanz, Konstanz 78457, Germany*

(Dated: April 12, 2025)

## SUPPLEMENTAL MATERIAL

### Materials and Methods

*Liquids and silicone gels.*—As gels, we used two different kinds of silicones, obtained from Gelest and Dow Corning, respectively. For Gelest materials, we used custom formulations inspired by [1, 2], based on a vinyl-end-functionalized PDMS prepolymer (DMS-V31, Gelest) and two different methylhydrosiloxane-dimethylsiloxane copolymers (HMS-053 and HMS-082, Gelest) as cross-linker, and a platinum-complex catalyst (SIP6831.2, Gelest) to get zero-frequency storage modulus $G_0 \sim 1.7\,\mathrm{kPa}$. We first prepared two stock mixtures, base and catalyst (component A), and base and cross-linker (component B), in proportions that the desired ratio of base polymer to cross-linker in the final gel formulation was achieved by mixing components A and B at a mass ratio of 9:1; For Dow Corning CY52-276A/B (Dow), we mixed components A and B in a mass ratio of 1:1, to obtain $G_0 \sim 1.3\,\mathrm{kPa}$. The preparation procedure is analogous to Refs. [2, 3]. As liquid droplets, we used ethylene glycol (EG, Sigma, purity $\geq 99\%$).

*Preparation of gels on a rubber.*—The stiff holder ($\sim 65 \times 65 \times 5\,\mathrm{mm}$) was made of polyvinyl siloxane (PVS) elastomer (Elite Double 22, Zhermack) by mixing equal quantities of catalyst and base liquids, degassed in a vacuum, and then cured at $75\,^\circ\mathrm{C}$ in an oven for 4 hours to obtain $G_0 \sim 100\,\mathrm{kPa}$. Additionally, a $30 \times 26 \times 1.3$ mm rectangular trough was molded into the central part of one side of the PVS to control the thickness of the soft gel layer. This PVS rubber was clamped in an expansion device and pre-stretched by at least 50%. The degassed mixture of silicone oils was then poured into the trough on the pre-stretched PVS support, left on an optical table to flatten for 4 hours and then cured at $75\,^\circ\mathrm{C}$ for 24 hours, covered by a glass plate to avoid dust contamination. To mitigate long-term material trends, the covered sample was stored inside a clean hood for over a week prior to use.

*Sliding droplet experiments.*— The pre-strain $\epsilon$ of the soft gel is set by either applying additional stretching ($\epsilon > 0$) or partially releasing ($\epsilon < 0$) the pre-stretched gel-PVS bilayer; Here, $\epsilon$ is determined by the marker displacement of stretcher, which is measured with a micrometer [4, 5]. The pre-strain was applied quasistatically, with each change in strain followed by at least 30 min for relaxation prior to the next adjustment. For each strain, around 5 EG droplets with a defined volume were carefully pipetted ($2-20\,\mu\mathrm{L}$ and $0.05-2\,\mu\mathrm{L}$, Gilson micro-pipette) onto the center region of soft gels. After the droplets reached equilibrium ($\sim 30$ min), its profile was imaged for estimating actual volume, and then the setup was rotated by $90^\circ$ so that gravity drives the sliding motion. The droplets were recorded by a digital camera (1-10 fps, PointGray Grasshopper2) attached to a telecentric lens (1.0x, working distance 62.2 mm, Thorlabs) or a macro lens (Nikon AF Micro Nikkor 60 mm f=2:8D), illuminated in reflection by a ring light (Amscope). To minimize the uncertainty of the droplet volume, we used the footprint diameter and the contact angle to calculate the volume of each droplet after reaching equilibrium, i.e., before rotating the setup, and then only considered those with a volume deviation of less than $0.05\,\mu\mathrm{L}$. For clarity, we only present four typical groups of experimental data in Fig. 2 of the main manuscript. Note that for large droplets, there is no change of the contact angle with the applied strain [1, 2], the angle of EG droplets on the silicone gel always re-equilibrates to a same value, namely $\theta \approx 85^\circ$.

*On-site rheological measurements.*— First, an annular Teflon plate with thickness of 2 mm, outer diameter of 60 mm and inner diameter of 25 mm was fabricated as a mold. Then, the Teflon plate was attached on a PVS rubber sheet (without a trough); The un-cured silicone gel mixture was poured on the reservoir formed by the annular plate and the rubber sheet, left on an optical table for a few hours, and cured at $75\,^\circ\mathrm{C}$ for 24 hours. Note that the gel was prepared with the same protocol of that in the sliding droplet experiments. Finally, the sample placed in a rheometer (MCR 502, Anton Paar, PP25) and continuously measured for over two weeks.

All experimental data was analyzed by standard image correlation techniques in custom-made Python code and/or the open-source software ImageJ.

## Descriptions of Movies

**Movie S1**: 5 µL EG droplets sliding down a gel (Dow, $\sim 1.3$ kPa) with $\epsilon = 0.23, 0, -0.18$, and $-0.22$. The movie plays at 20× real time.

**Movie S2**: A 1 µL EG droplet sliding down a creased gel (Dow, $\sim 1.3$ kPa), exhibiting a "run-and-stop" motion. The movie plays at 500× real time.

## "Run-and-stop" motion of droplets on creased soft gels

Fig. S1(a) shows "run-and-stop" motion of droplets with three different sizes, 2 µL, 1 µL, and $\sim 0.2$ µL; For a very small droplet with volume of $\sim 0.2$ µL, a complete pinning can be observed (Fig. S1b). Fig. S2(a) and S2(b) illustrates that when a horizontally placed gel (Dow, $\sim 1.1$ kPa) is consecutively compressed, creasing first forms near the three-phase contact line of the sessile droplet.

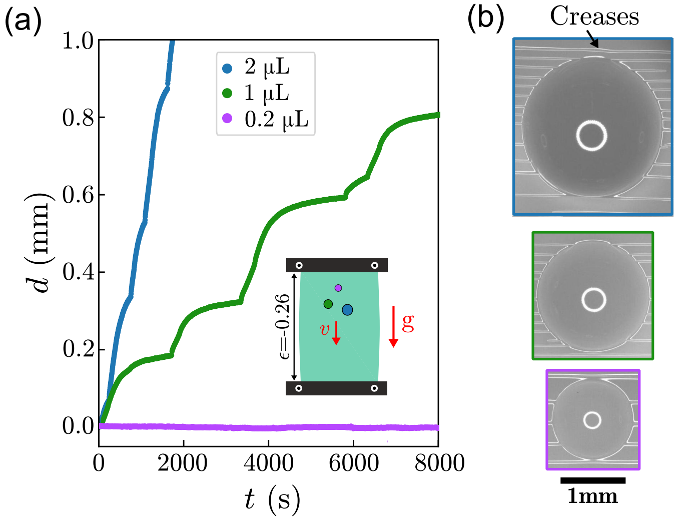


FIG. S1. Three small-sized EG droplets (2 µL, 1 µL, and $\sim 0.2$ µL) sliding down a creased gel surface ($\epsilon \sim -0.26$, Dow, $\sim 1.3$ kPa). (a) Sliding distance $d$ *vs* time $t$ for: "Run-and-Stop" motions for droplets of 2 µL and 1 µL; Complete pinning for an even smaller droplet of $\sim 0.2$ µL. Inset shows the position where three droplet profiles in (b) are captured. (b) Profiles showing the sliding droplets with: volumes of 2 µL, 1 µL, and $\sim 0.2$ µL from the top to bottom panels, respectively.

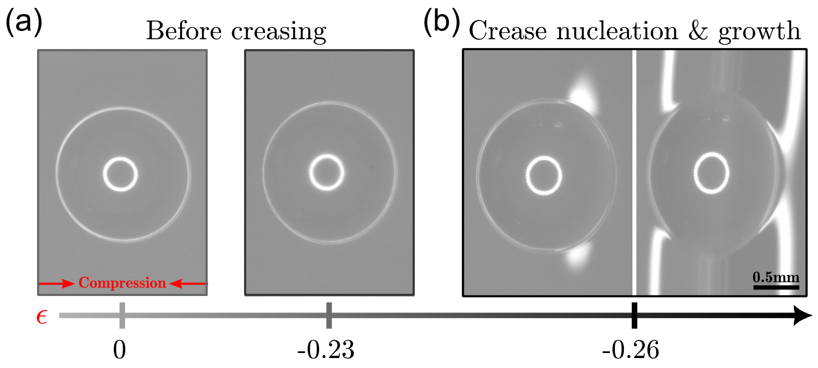


FIG. S2. Crease forming under a sessile EG droplet during compression (Dow, $\sim 1.1$ kPa). (a) Before creasing: the droplet is sitting on a compressed gel with $\epsilon \sim -0.23$, and (b) during creasing: the crease first appears under the droplet with $\epsilon \sim -0.26$, and grows beyond it.

### Anisotropic motion and aspect ratios of sliding droplets

Fig. S3 illustrates the droplet sliding speed $v$ *vs* pre-strain $\epsilon_{||}$, i.e., the strain parallel to the direction of droplet motion, for experimental data in Figs. 2(b) and 3(a) of the main manuscript; Note that the case of droplets sliding perpendicular to the stretched direction (solid purple circles) is also included. Fig. S4 shows aspect ratios, defined as the ratio of droplet's length to width, corresponding to experiments in Figs. 2(b) and 3(a) of the main manuscript.

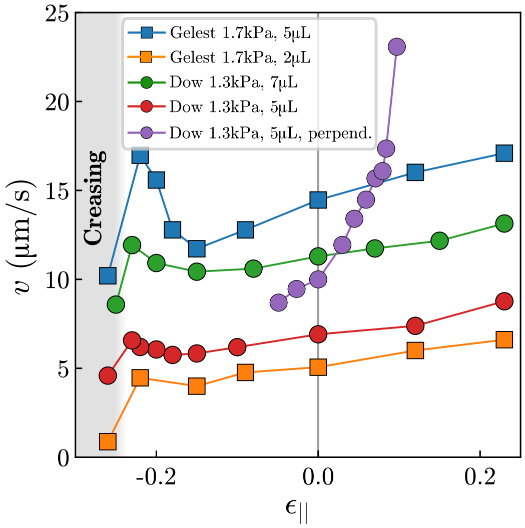


FIG. S3. Droplet sliding speed $v$ *vs* pre-strain $\epsilon_{||}$ in the direction parallel to the droplet motion. Note that the case of droplets sliding perpendicular to the stretched direction (solid purple circles) is also included.

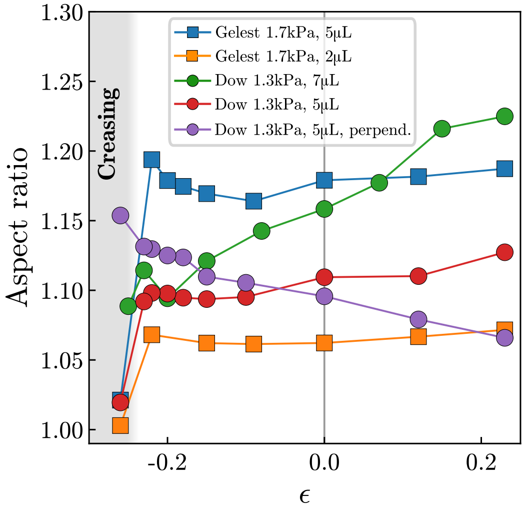


FIG. S4. Aspect ratios of sliding droplets corresponding to experiments in Figs. 2(b) and 3(a) of the main manuscript.

**Incremental elasticity of pre-strained elastic layers**

The equilibrium condition for the incremental stress $s_{ij}$ on top of a finite, homogeneous, shear-free pre-stress is given by [6]

$$\partial_x s_{11} + \partial_y s_{12} - P\,\partial_y \xi = 0, \tag{S1a}$$
$$\partial_x s_{12} + \partial_y s_{22} - P\,\partial_x \xi = 0, \tag{S1b}$$

where direction 1 is parallel to the free surface, and direction 2 perpendicular, increasing into the elastic material. There shall be no incremental strain in direction 3 (plane strain). Here, $P$ is the initial pre-stress in the solid, given by the normal stress difference of the pre-strained state, namely, $P = S_{22} - S_{11}$, and $\xi$ is the rotation, due to the incremental displacement field $(u_1, u_2)$, in directions 1 and 2, respectively. The incremental strains $\epsilon_{11}$, $\epsilon_{22}$, $\epsilon_{12}$ and the rotation $\xi$ are

$$\epsilon_{11} = \partial_x u_1, \tag{S2a}$$
$$\epsilon_{22} = \partial_z u_2, \tag{S2b}$$
$$\epsilon_{12} = \frac{1}{2}\left(\partial_x u_2 + \partial_z u_1\right), \tag{S2c}$$
$$\xi = \frac{1}{2}\left(\partial_x u_2 - \partial_z u_1\right). \tag{S2d}$$
$$\tag{S2e}$$

The incremental stress-strain relation is

$$s_{ij} = 2\mu\epsilon_{ij} + s\,\delta_{ij}, \tag{S3}$$

with the incremental shear modulus

$$\mu = \frac{G_0}{2}\left(\lambda_1^2 + \lambda_2^2\right), \tag{S4}$$

where $\lambda_1$ and $\lambda_2$ are the (principal) pre-stretches in directions 1 and 2, respectively (see Fig. S5).

The solid pre-stress is related to the stretches by

$$P = S_{22} - S_{11} = G_0\left(\lambda_2^2 - \lambda_1^2\right). \tag{S5}$$

The surface (located at $z = 0$) boundary conditions are

$$s_{12}\big|_{z=0} = 0, \tag{S6a}$$
$$s_{22}\big|_{z=0} = t_2(x), \tag{S6b}$$

where $t_2$ is the normal traction. To derive the Green's function, the traction is assumed sinusoidal:

$$t_2(x) = t_q\,\cos qx. \tag{S7}$$

The ansatz for the incremental displacements,

$$u_1 = \left(A\,e^{\alpha z} + C\,e^{\gamma z}\right)\sin qx, \tag{S8a}$$
$$u_2 = \left(B\,e^{\alpha z} + D\,e^{\gamma z}\right)\cos qx, \tag{S8b}$$

contains two exponentials with different coefficients to $z$ in the exponent, required due to appearance of the rotation $\xi$ in the equilibrium condition Eq. (S1). Inserting Eq. (S8) into Eqs. (S2) and (S3), and further into Eqs. (S1) and (S6) gives $A$, $B$, $C$, $D$, $\alpha$, and $\gamma$. With the pre-compression coefficient

$$\zeta = \frac{P}{2\mu} = \frac{\lambda_2^2 - \lambda_1^2}{\lambda_2^2 + \lambda_1^2}, \tag{S9}$$

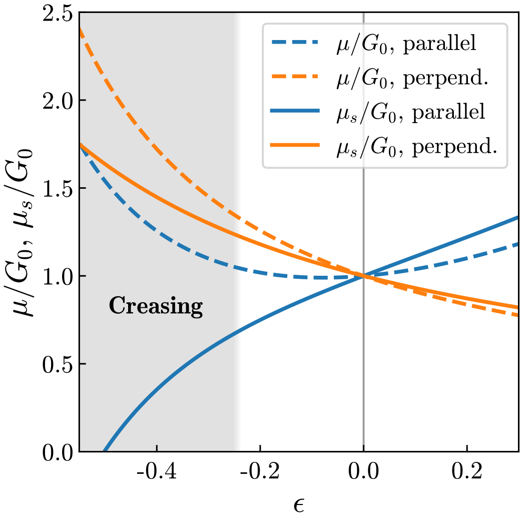


FIG. S5. Scaled effective shear modulus $\mu/G_0$ and scaled surface modulus $\mu_s/G_0$ as a function of pre-strain $\epsilon$ in parallel and perpendicular, respectively. The region of the crease-instability is indicated by the gray shade. Note that $\mu$ is non-monotonic for the parallel pre-strain $\epsilon_{||}$ (dashed blue line), increasing by $\sim 15\%$ toward the edges of the experimentally investigated range of $\epsilon$, while $\mu_s$ depends monotonically on $\epsilon$, vanishing at a critical compression (solid blue line).

and the shorthand

$$k = \sqrt{\frac{1-\zeta}{1+\zeta}} = \frac{\lambda_1}{\lambda_2}, \tag{S10}$$

the obtained combinations of exponent coefficients are

$$\alpha_1 = q \qquad \gamma_1 = -q, \tag{S11a}$$
$$\alpha_1 = q \qquad \gamma_2 = k\,q, \tag{S11b}$$
$$\alpha_1 = q \qquad \gamma_3 = -k\,q, \tag{S11c}$$
$$\alpha_2 = -q \qquad \gamma_2 = k\,q, \tag{S11d}$$
$$\alpha_2 = -q \qquad \gamma_3 = -k\,q, \tag{S11e}$$
$$\alpha_3 = k\,q \qquad \gamma_3 = -k\,q. \tag{S11f}$$

Exchanging $\alpha$ and $\gamma$ yields redundant expressions, and $\alpha_2 = \gamma_1$, $\alpha_3 = \gamma_2$, so the four remaining exponents can be combined into a displacement field with two unknowns. For the half-space case, solved in Ref. [6], only decaying functions of $y$ are admissible, eliminating all but negative exponents. For a layer of finite thickness, all exponents are possible, and the bottom boundary condition

$$u_1\big|_{z=h_0} = 0, \tag{S12a}$$
$$u_2\big|_{z=h_0} = 0, \tag{S12b}$$

selects the remaining unknowns.

In the limit $k \to 1$, one recovers the displacements without pre-stress [7]. The Green's function $K_{22}(q)$ is obtained by evaluating $u_2$ at $z = 0$ and eliminating $t_q \cos qx$:

$$K_{22}(q) = \frac{1}{2\mu q} \frac{(k^4-1)\,(k\cosh(kqh_0)\sinh(qh_0) - \cosh(qh_0)\sinh(kqh_0))}{k(5+2k^2+k^4)\cosh(qh_0)\cosh(kqh_0) - (1+6k^2+k^4)\sinh(qh_0)\sinh(kqh_0) - 4k(1+k^2)}. \tag{S13}$$

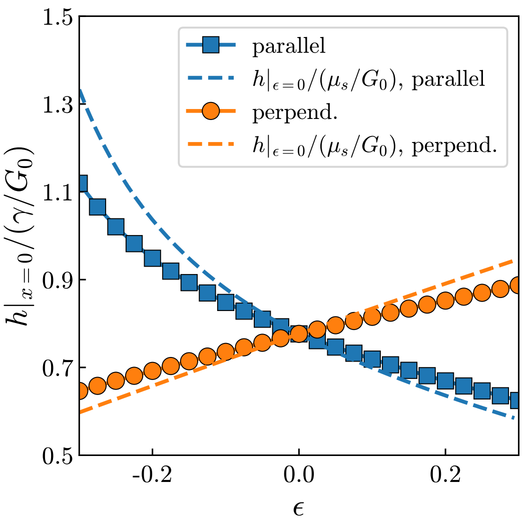


FIG. S6. Ridge height $h|_{x=0}$ scaled by $\gamma/G_0$ as a function of the applied pre-strain $\epsilon$ (symbols), compared to the scaling expected from the effective modulus $\mu_s/G_0$ for an elastic half-space (dashed lines).

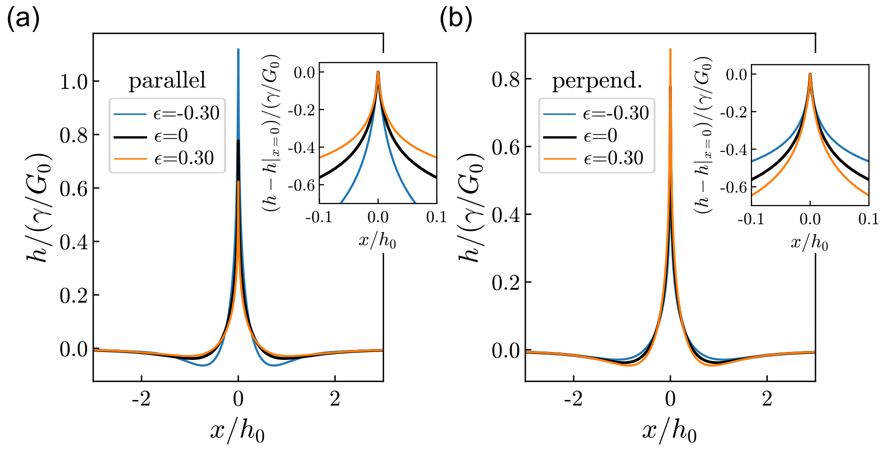


FIG. S7. Profiles calculated according to Eq. (S14) for the cases with a primary pre-stretch $\epsilon$ parallel (a) and perpendicular (b) to the $x$-axis. Here, $h_0 \sim 1.3$ mm, $\gamma_s \sim 18$ mN/m, $G_0 \sim 1.34$ kPa. Insets: Zoomed views of wetting ridges near the tip.

To obtain the profiles of wetting ridge, the inverse Fourier transform

$$h(x) = \frac{\gamma \sin\theta}{\pi} \int_0^\infty dq \, \frac{\cos qx}{K_{22}(q)^{-1} + \gamma_s q^2}, \tag{S14}$$

is evaluated numerically [8], where $\gamma_s$ is the solid surface tension. Fig. S6 shows the ridge height on a finite thickness layer as a function of pre-strain, compared to the scaling of the effective surface modulus $\mu_s$ for an elastic half-space (see Fig. S5). On a finite thickness layer, the height dependence is slightly reduced as compared to the scaling with $\mu_s$. Fig. S7(a) and S7(a) shows the resulting profiles at the front or rear of the droplet for the case of sliding parallel and perpendicular to the applied pre-strain, respectively.

## Long-term trends in the material parameters

To analyze possible long-term trends in the rheology of our gel while in contact with the PVS support, we perform on-site measurements of a silicone gel (Dow, $\sim 1.3$ kPa) sample that is cured on the top of a PVS rubber by the rheometer, continuously monitored for over two weeks (see Fig. S8). We fit the storage modulus $G'$ and loss modulus

$G''$ of the soft gel by a power-law model [9, 10]

$$G(\omega) = G'(\omega) + iG''(\omega) = G_0[1 + (\omega\tau)^n], \tag{S15}$$

where $\omega$ is the angular frequency, $G_0$ the storage modulus at zero frequency, $\tau$ relaxation timescale, and $n$ rheological exponent. A representative viscoelastic response of the gel measured on Day 7 is illustrated in Fig. S9(a). We notice that the gel rheology, as characterized by $G_0$, $\tau$ and $n$, becomes stable after about one week, yielding $G_0 \to 1.34\,\text{kPa}$, $\tau \to 0.066\,\text{s}$, and $n \to 0.59$ (Fig. S9b).

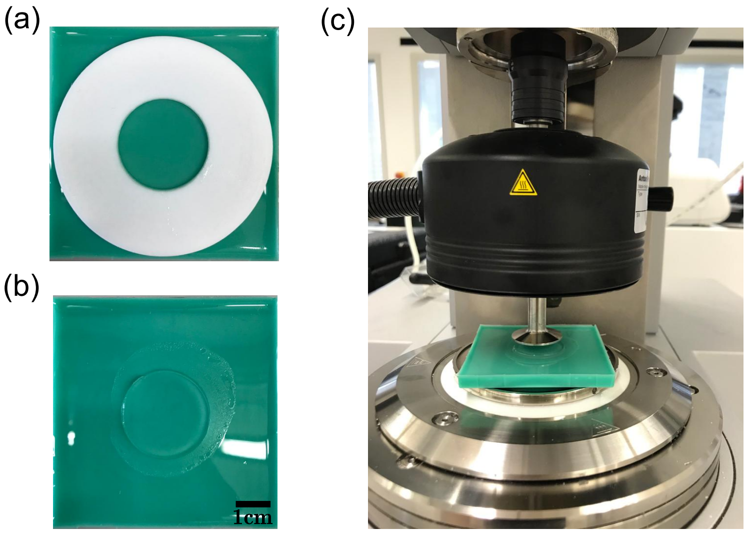


FIG. S8. The protocol showing on-site rheological measurements of soft gels on a thick, stiff PVS layer: (a,b) Sample preparation: a soft silicone gel (transparent, Dow, $\sim 1.3\,\text{kPa}$) cured on the top of a PVS rubber (green); The liquid gel prepolymer is first confined in an annular Teflon plate (a), which is removed after curing (b). (c) Sample measurement: the silicone gel-PVS bilayer is continuously measured under the rheometer for over two weeks.

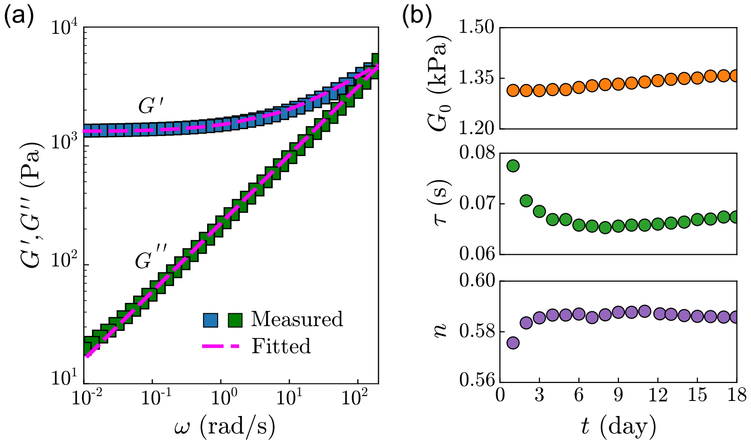


FIG. S9. On-site rheological measurements of a soft silicone gel (Dow, $\sim 1.3\,\text{kPa}$) on the top of a stiff PVS-rubber support, continuously monitored by a rheometer for over two weeks. (a) The complex moduli $G$ can be fitted by a power-law rheological model, with $G'$ and $G''$ the storage and loss moduli, respectively. (b) The dependence of rheological parameters $G_0$, $\tau$, and $n$ on time (day). Rheology becomes stable after around one week, indicating that the migration of extractables from the silicone gel into the PVS support has reached an equilibrium state.

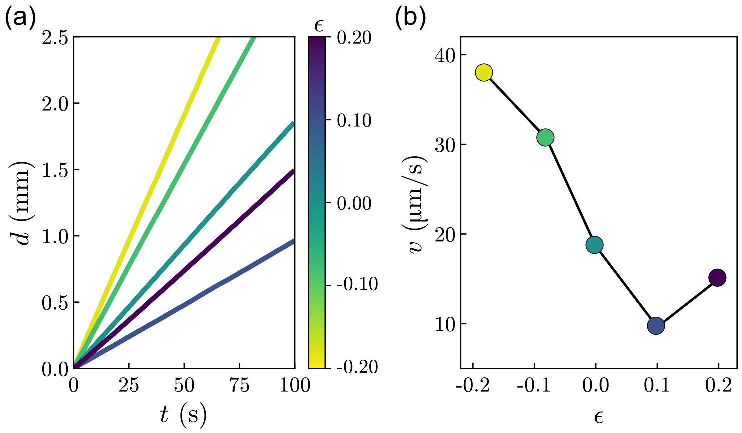


FIG. S10. Droplets (5 µL) sliding down a ∼1.3 kPa Dow gel immediately after preparation: (a) Position $d$ *vs* time $t$, and (b) speed $v$ *vs* pre-strain $\epsilon$. Compared to the aged samples (Fig. 2 of the main manuscript), velocities are larger, especially in the compressive regime.

---

* ychao@hit.edu.cn; Present address: School of Energy Science and Engineering, Harbin Institute of Technology, Harbin 150001, China
† stefan.karpitschka@uni-konstanz.de

[1] Q. Xu, K. E. Jensen, R. Boltyanskiy, R. Sarfati, R. W. Style, and E. R. Dufresne, Direct measurement of strain-dependent solid surface stress, Nature Communications **8**, 555 (2017).
[2] Q. Xu, R. W. Style, and E. R. Dufresne, Surface elastic constants of a soft solid, Soft Matter **14**, 916 (2018).
[3] H. Jeon, Y. Chao, and S. Karpitschka, Moving wetting ridges on ultrasoft gels, Physical Review E **108**, 024611 (2023).
[4] S. Mora, M. Abkarian, H. Tabuteau, and Y. Pomeau, Surface instability of soft solids under strain, Soft Matter **7**, 10612 (2011).
[5] M. A. J. van Limbeek, M. H. Essink, A. Pandey, J. H. Snoeijer, and S. Karpitschka, Pinning-induced folding-unfolding asymmetry in adhesive creases, Physical Review Letters **127**, 028001 (2021).
[6] M. A. Biot, Surface instability of rubber in compression, Applied Scientific Research **12**, 168 (1963).
[7] R. W. Style, R. Boltyanskiy, Y. Che, J. S. Wettlaufer, L. A. Wilen, and E. R. Dufresne, Universal deformation of soft substrates near a contact line and the direct measurement of solid surface stresses, Physical Review Letters **110**, 066103 (2013).
[8] S. Karpitschka, S. Das, M. van Gorcum, H. Perrin, B. Andreotti, and J. H. Snoeijer, Droplets move over viscoelastic substrates by surfing a ridge, Nature Communications **6**, 7891 (2015).
[9] H. H. Winter and F. Chambon, Analysis of linear viscoelasticity of a crosslinking polymer at the gel point, Journal of Rheology **30**, 367 (1986).
[10] D. Long, A. Ajdari, and L. Leibler, Static and dynamic wetting properties of thin rubber films, Langmuir **12**, 5221 (1996).
